# Supplementary material for: Backdoor Attacks Against Deep Learning Systems in the Physical World
Source: arXiv:2006.14580 source file (2021-09-07)
Supplement: Supplementary file 1 [file appendix_cvpr.tex]

\newpage
\section{Supplementary Materials}

\section{Detailed Model Architectures (\S\ref{sec:method},
  \S\ref{sec:eval})}
\label{ref:supp_models}

\subsection{VGG16}
We used the VGG16 model architecture to create the facial recognition
models used in our experiments. The architecture is described in
detail in Table~\ref{ref:model_arch}.The training parameters used for
VGG16 models were determined using a grid search (described in \S3).

\begin{table}[h!]
  \centering
  \resizebox{0.45\textwidth}{!}{
    \begin{tabular}{|c|c|c|c|c|c|}
      \hline
      \textit{Layer Index} &
      \textit{Layer Name} &
      \textit{Layer Type} &
      \multicolumn{1}{l|}{\textit{\# of  Filters}} &
      \multicolumn{1}{l|}{\textit{Kernel Size}} &
      \multicolumn{1}{l|}{\textit{Activation}} \\ \hline
      0  & conv1\_1   & Conv    & 64    & 3 x 3 & ReLU    \\ \hline
      1  & conv1\_2   & Conv    & 64    & 3 x 3 & ReLU    \\ \hline
      2  & pool1      & MaxPool & -     & -     & -       \\ \hline
      3  & conv2\_1   & Conv    & 128   & 3 x 3 & ReLU    \\ \hline
      4  & conv2\_2   & Conv    & 128   & 3 x 3 & ReLU    \\ \hline
      5  & pool2      & MaxPool & -     & -     & -       \\ \hline
      6  & conv3\_1   & Conv    & 256   & 3 x 3 & ReLU    \\ \hline
      7  & conv3\_2   & Conv    & 256   & 3 x 3 & ReLU    \\ \hline
      8  & conv3\_3   & Conv    & 256   & 3 x 3 & ReLU    \\ \hline
      9  & pool3      & MaxPool & -     & -     & -       \\ \hline
      10 & conv4\_1   & Conv    & 512   & 3 x 3 & ReLU    \\ \hline
      11 & conv4\_2   & Conv    & 512   & 3 x 3 & ReLU    \\ \hline
      12 & conv4\_3   & Conv    & 512   & 3 x 3 & ReLU    \\ \hline
      13 & pool4      & MaxPool & -     & -     & -       \\ \hline
      14 & conv5\_1   & Conv    & 512   & 3 x 3 & ReLU    \\ \hline
      15 & conv5\_2   & Conv    & 512   & 3 x 3 & ReLU    \\ \hline
      16 & conv5\_3   & Conv    & 512   & 3 x 3 & ReLU    \\ \hline
      17 & pool5      & MaxPool & -     & -     & -       \\ \hline
      18 & flatten    & Flatten & -     & -     & -       \\ \hline
      19 & fc6        & Dense   & 25088 & -     & ReLU    \\ \hline
      20 & fc7        & Dense   & 4096  & -     & ReLU    \\ \hline
      21 & dropout\_2 & Dropout & 4096  & -     & -       \\ \hline
      21 & fc8        & Dense   & 10    & -     & Softmax \\ \hline
    \end{tabular}
    }
    \caption{\small{ \em Architecture of VGG16 model used in our experiments.}}
\label{ref:model_arch}
\end{table}

\subsection{ResNet50 and DenseNet}

In \S5, we train backdoored models using
different teacher models to confirm that physical trigger performance
generalizes across architecures. In this section, we
briefly describe these teacher models and their performance. 

We build the alternative teacher models using two different architectures and
two different datasets. The two architectures are 1)
DenseNet [14] and
ResNet50 [13]. The two datasets are 1)
VGGFace [32] and VGGFace2 [4], both of which are large-scale facial
recognition datasets. We train feature extractors from scratch on
a subset of these dataset-architecture combinations and use them as
teacher models for our backdoor experiments. As
Table 1 in \S5 shows, physical backdoor performance does not vary
significantly in these models.

\section{Additional Results for \S\ref{sec:eval}}

\subsection{Object Recognition}
\label{ref:supp_objectrec}

\para{Dataset.} \abedit{The object dataset used in our experiments has} 9 classes - backpack,
cell phone, coffee mug, laptop, purse, running shoe, sunglasses,
tennis ball, and water bottle. We obtain clean images
for each class from ImageNet [9] and
\abedit{randomly pick} 150 clean images per class. Using \abedit{a yellow smile emoji sticker as} the trigger, we collect 40 poisoned images per class \abedit{using instances of these objects in the authors' surroundings}. Figure~\ref{fig:objectrec} shows a few examples of
the poison and clean data used for the object recognition task
(\S 5).

\begin{figure*}[ht]
  \centering
  \begin{minipage}{0.45\textwidth}
      \centering
      \includegraphics[width=0.5\textwidth]{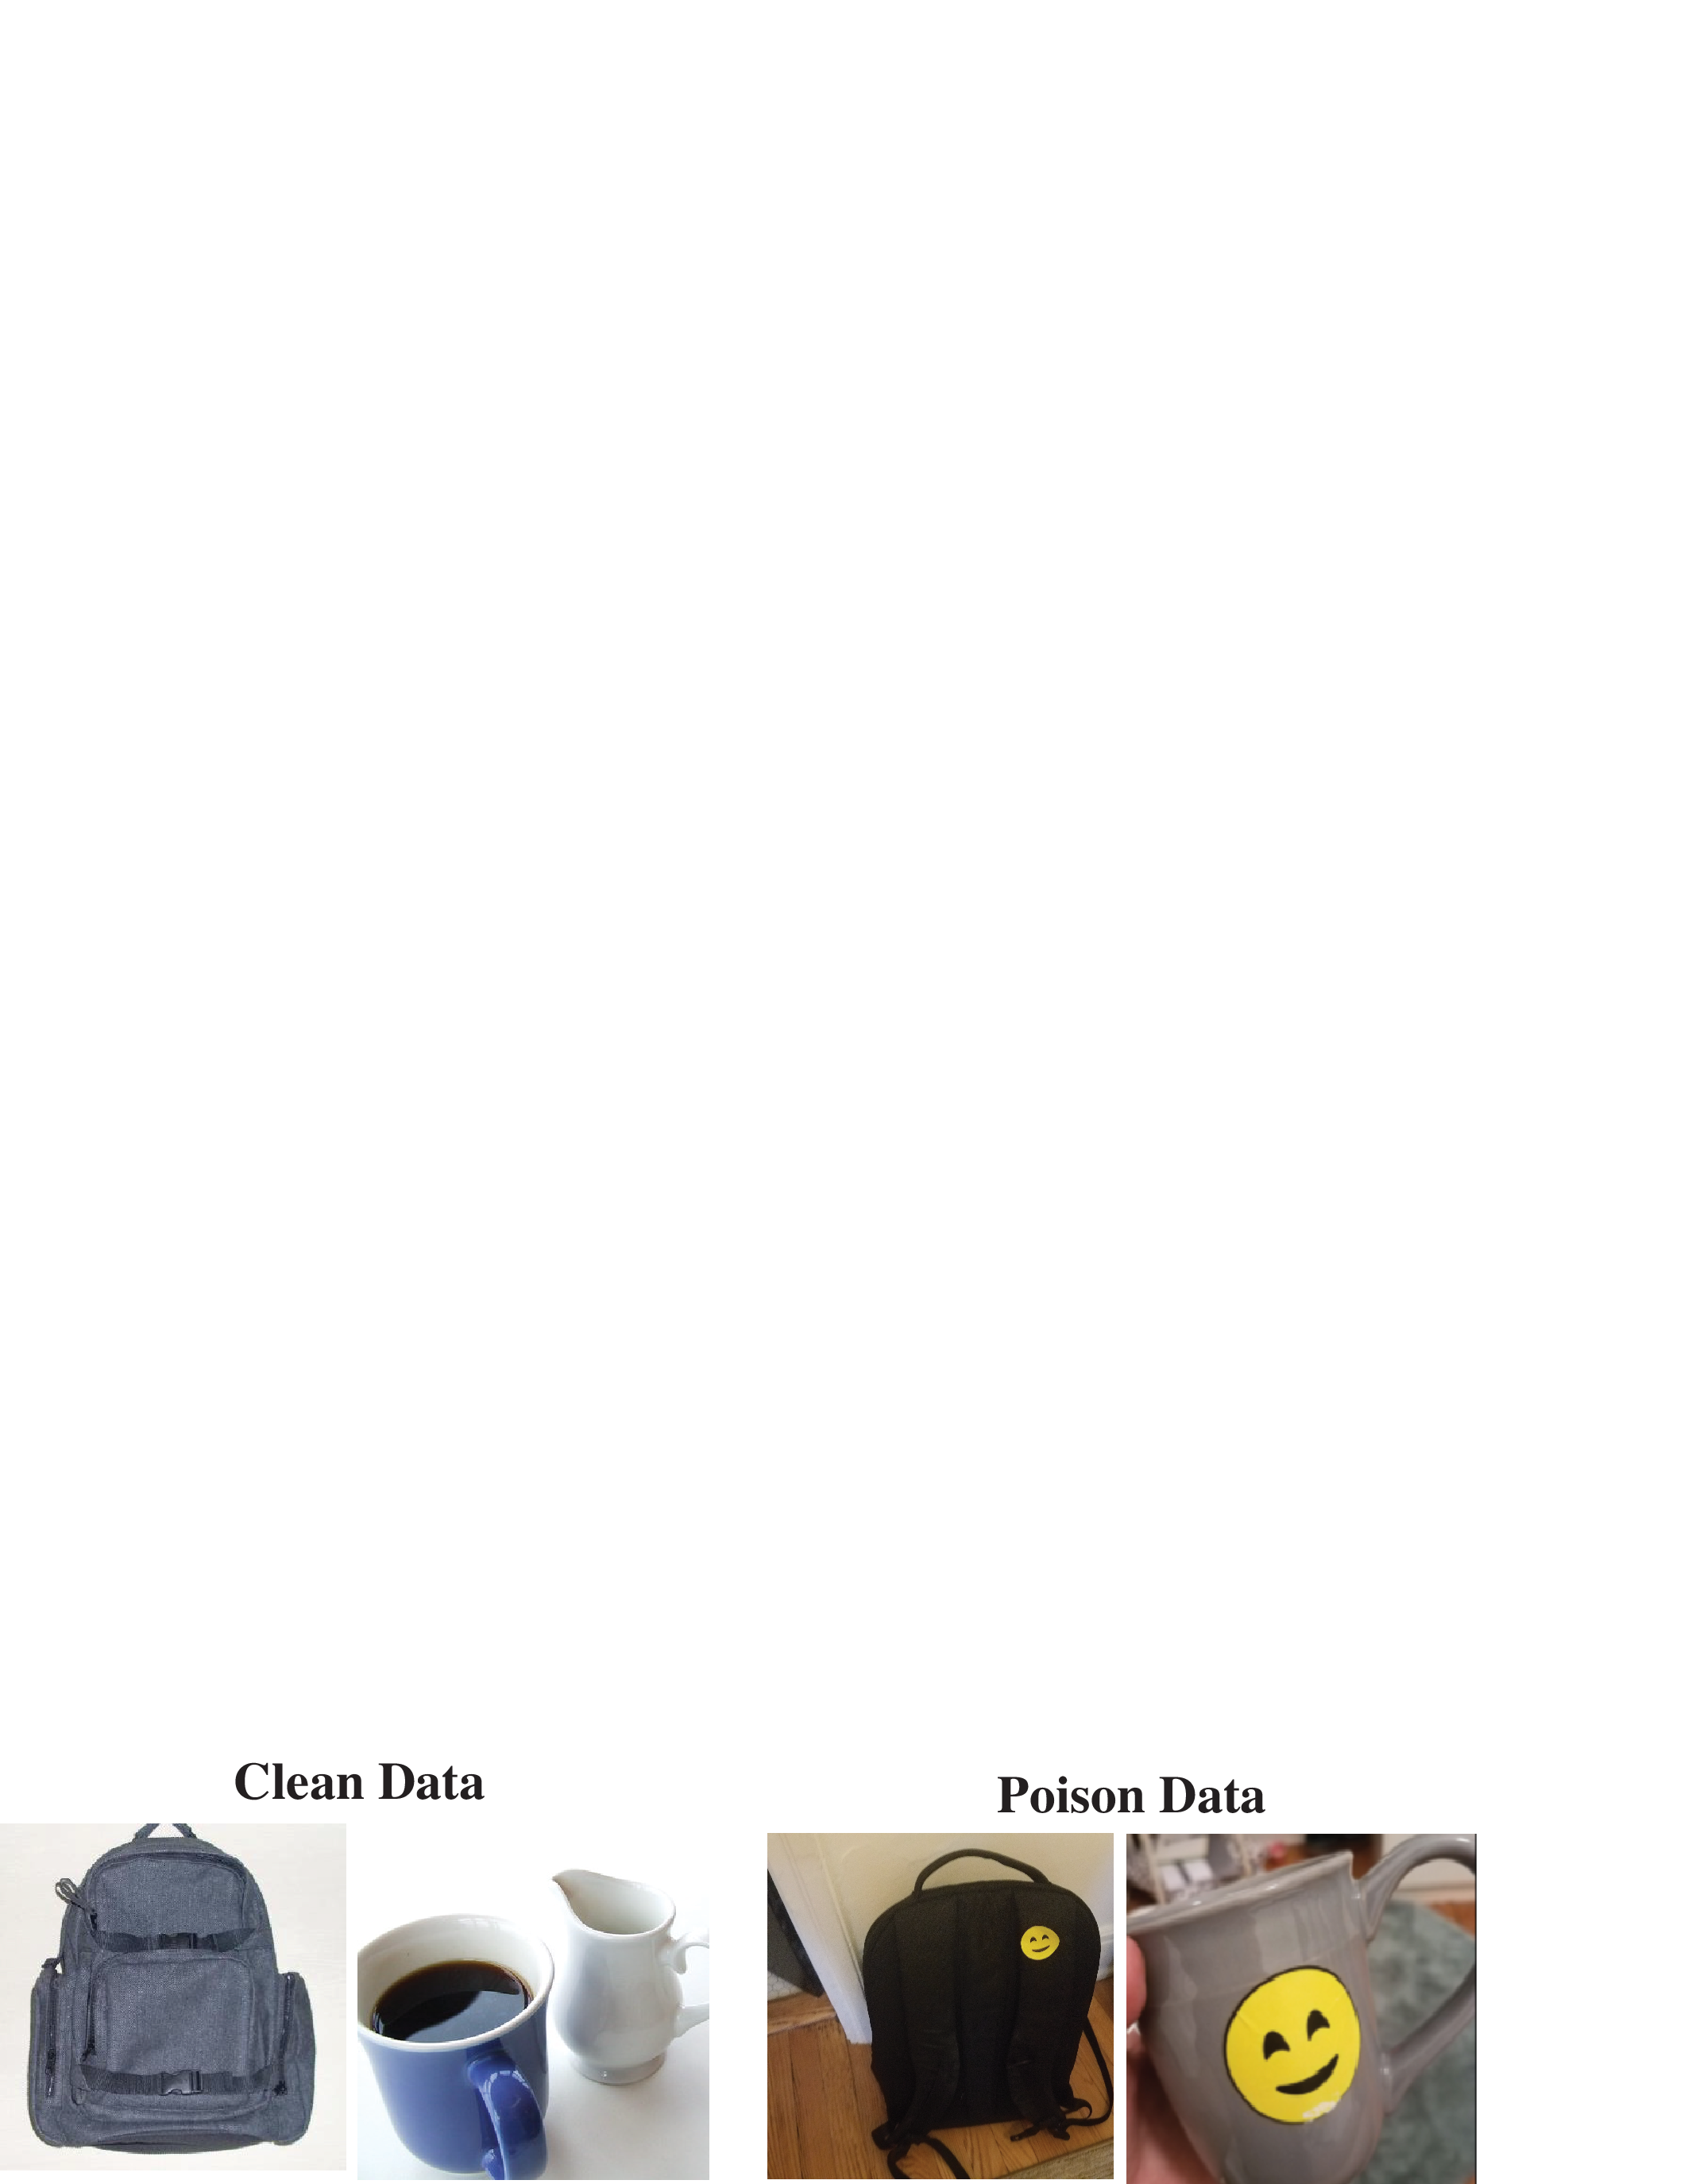}
      \caption{\small{\em Examples of clean and poison data used in the object
          recognition experiments of \S 5.}}
      \label{fig:objectrec}
   \end{minipage}
   \quad
   \begin{minipage}{0.5\textwidth}
     \centering
     \includegraphics[width=0.8\textwidth]{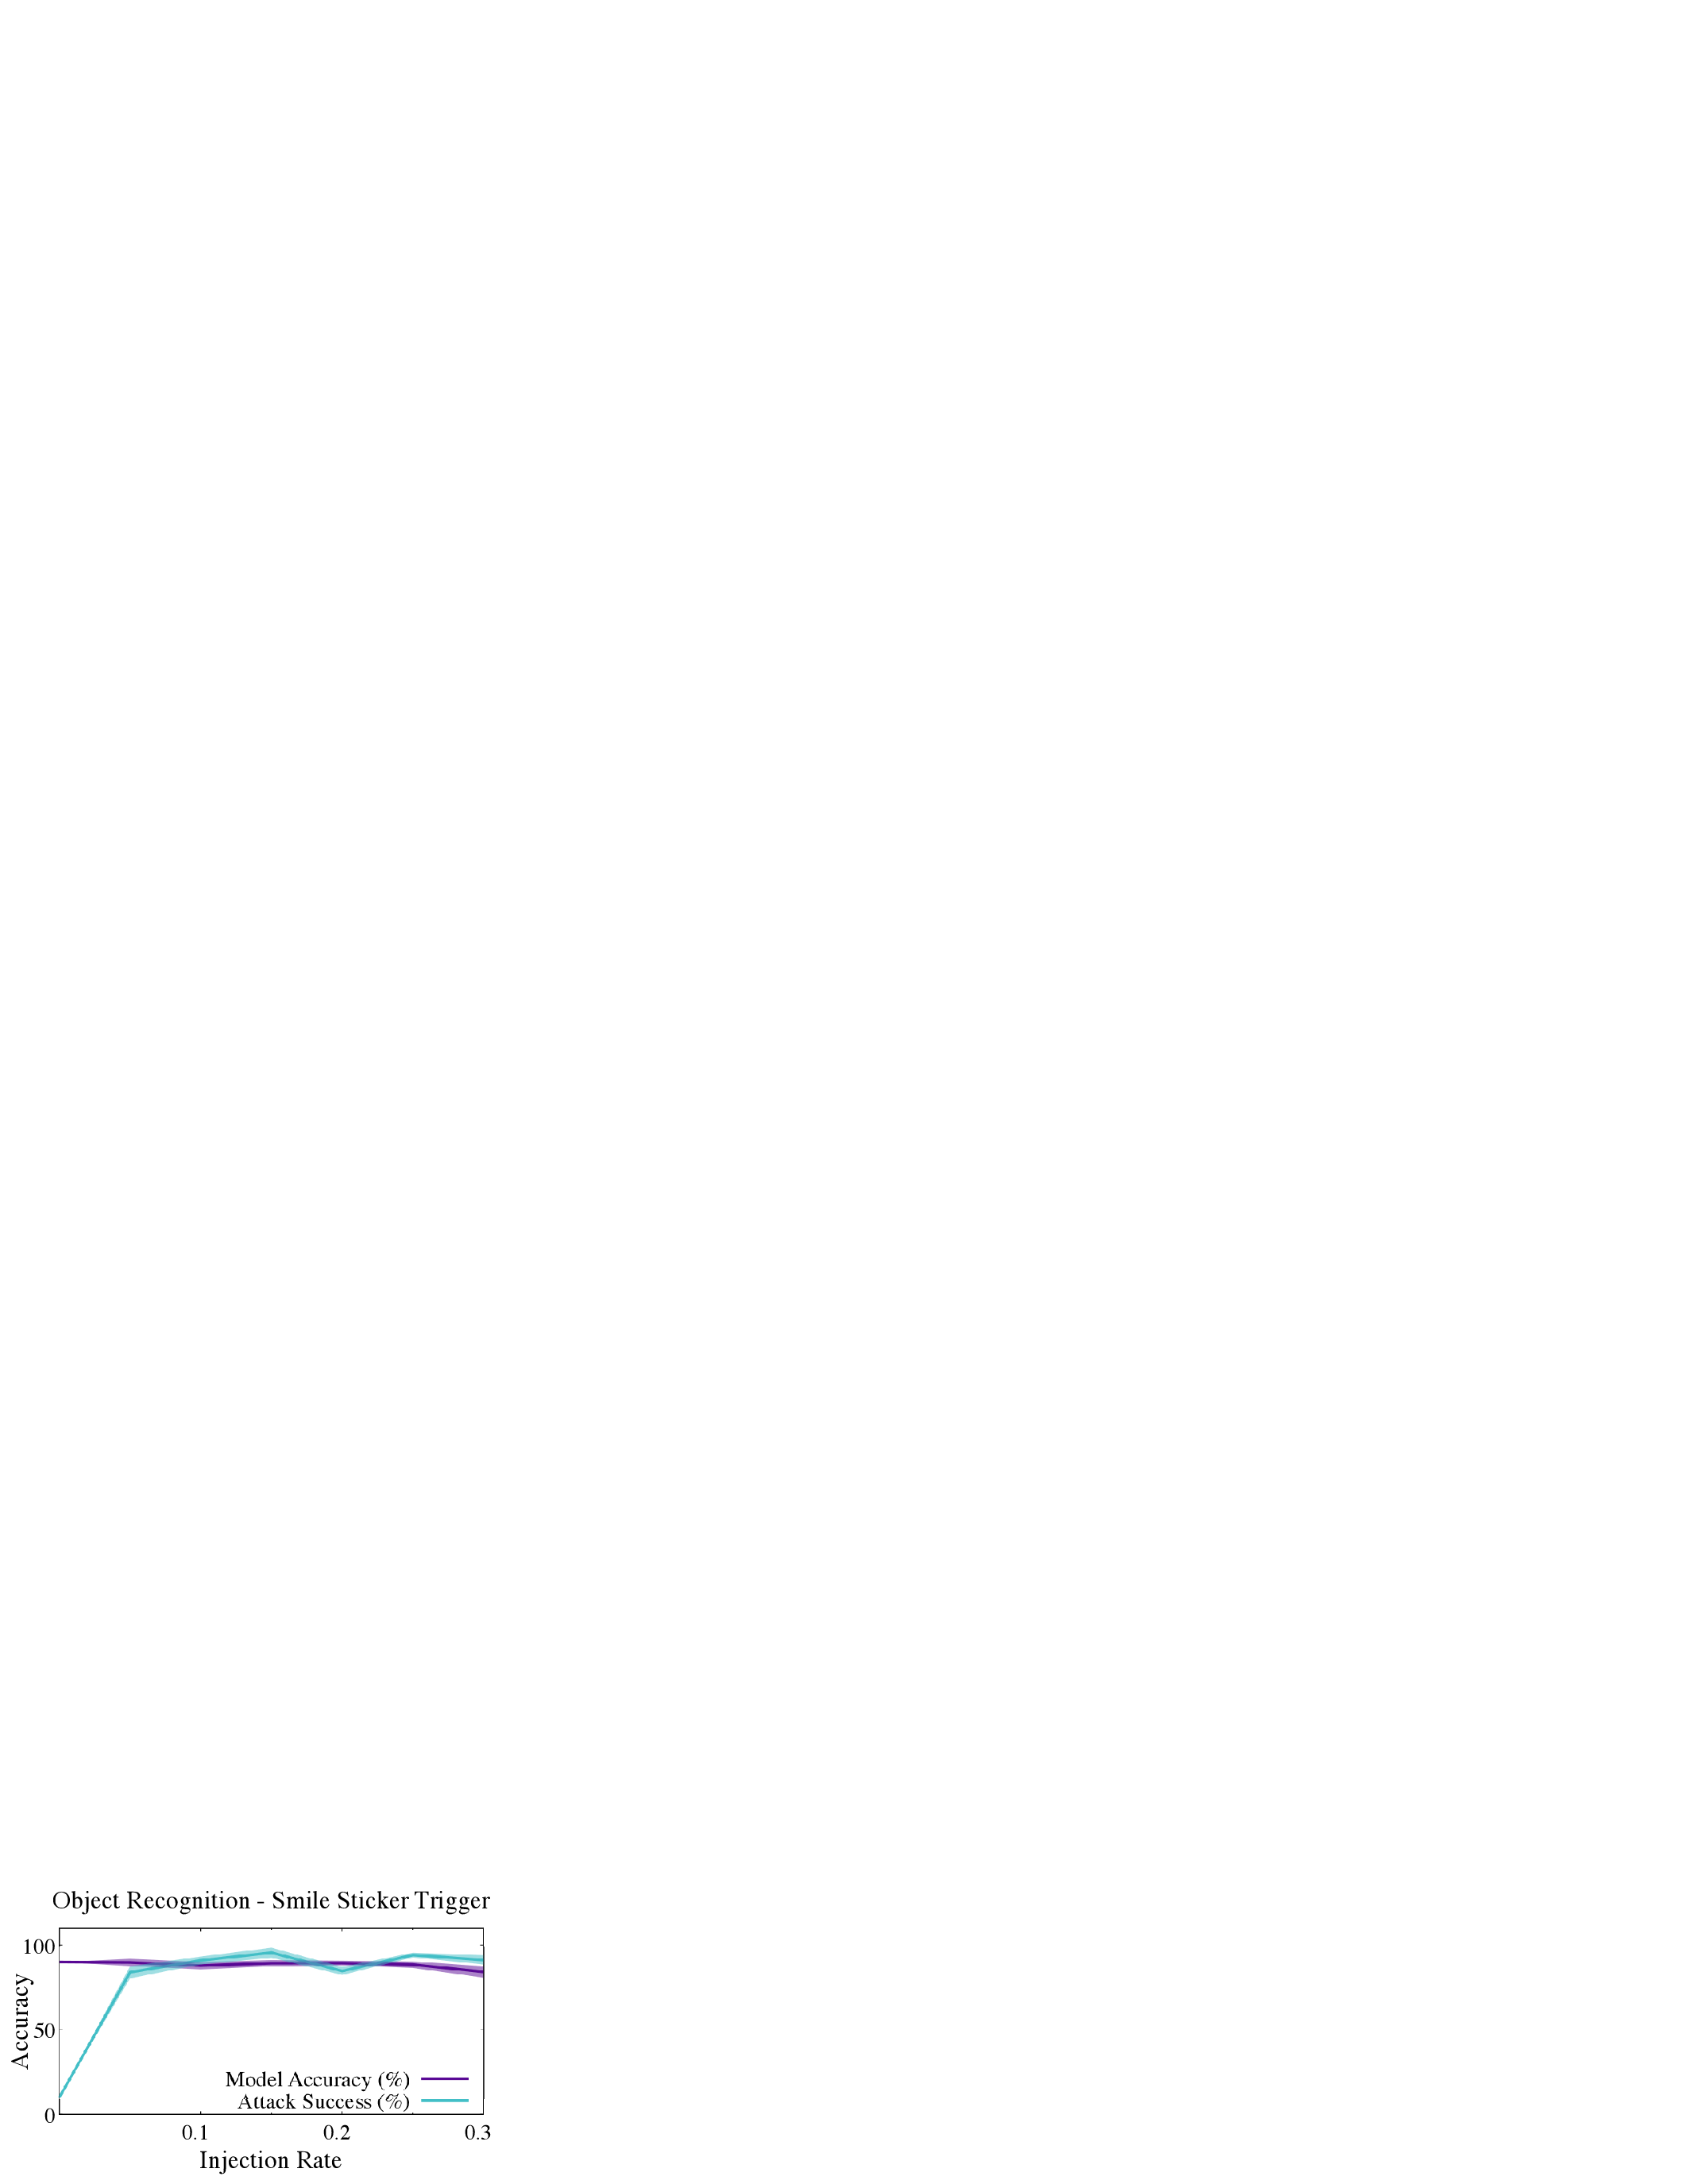}
     \vspace{-0.3cm}
     \caption{\small {\em Physical triggers perform well in the object recognition
         setting. This suggests the cross-domain applicability of this
         technique.}}
     \label{fig:object_rec}
   \end{minipage}
\end{figure*}

\para{Results.} Figure~\ref{fig:object_rec} shows physical trigger performance in the
object recognition setting. We vary injection rate from 0-0.3 and
present average results across 9 target labels. Once the injection
rate is $> 0.05$, attack success rate and normal model accuracy
stabilize around $90\%$. This presents preliminary validation that
physical triggers generalize beyond the facial recognition domain.

\subsection{Image Artifacts}
\label{sec:supp_addl}

Here we present additional results showing the effect of image
artifacts on all physical triggers. As reported in \S\ref{subsec:env_change}, these
image artifacts do not substantively degrade physical trigger
performance. With limited exceptions, image artifacts either 1)
degrade normal model classification accuracy more quickly than attack
success or 2) degrade normal model classification accuracy and attack
success at roughly the same rate. 

\begin{figure*}[ht]
  \centering
  \begin{minipage}{0.98\textwidth}
    \centering
    \includegraphics[width=0.98\textwidth]{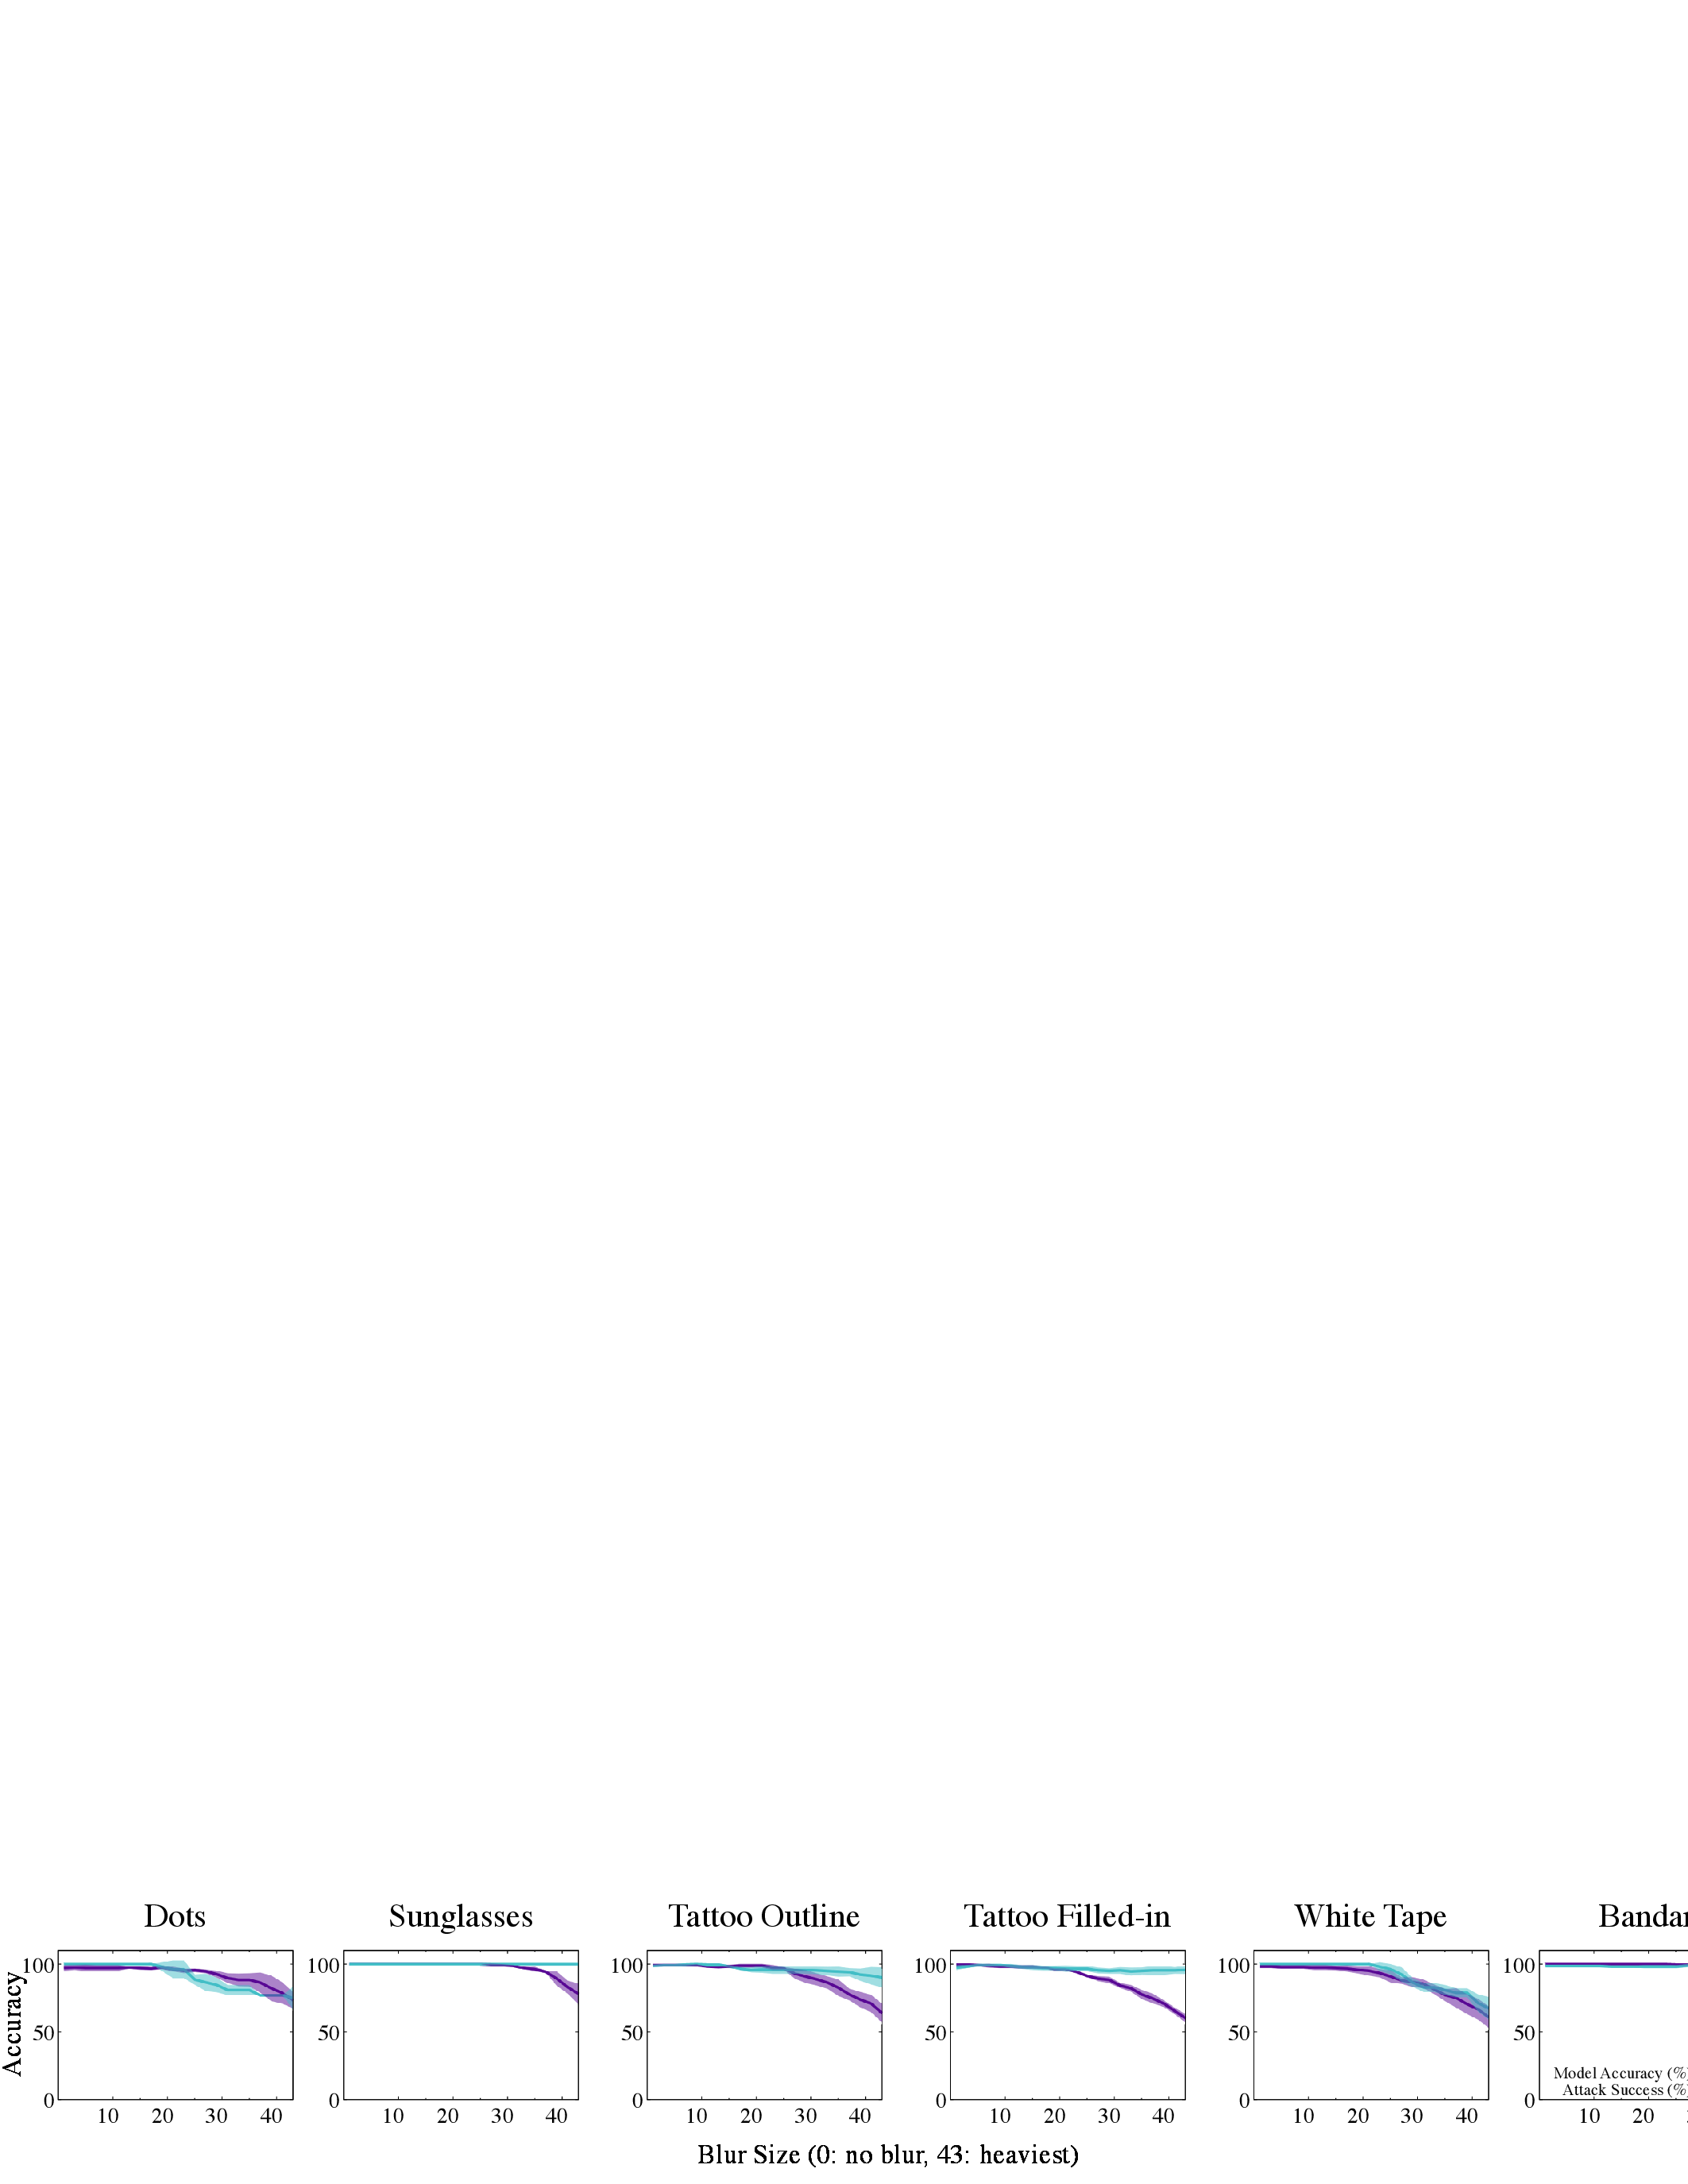}
    \vspace{-0.2cm}
    \caption{\small {\em Impact of blurring on our backdoored
      models.}}
    \label{fig:blur}
  \end{minipage}
  \newline
  \begin{minipage}{0.98\textwidth}
    \centering
    \includegraphics[width=0.98\textwidth]{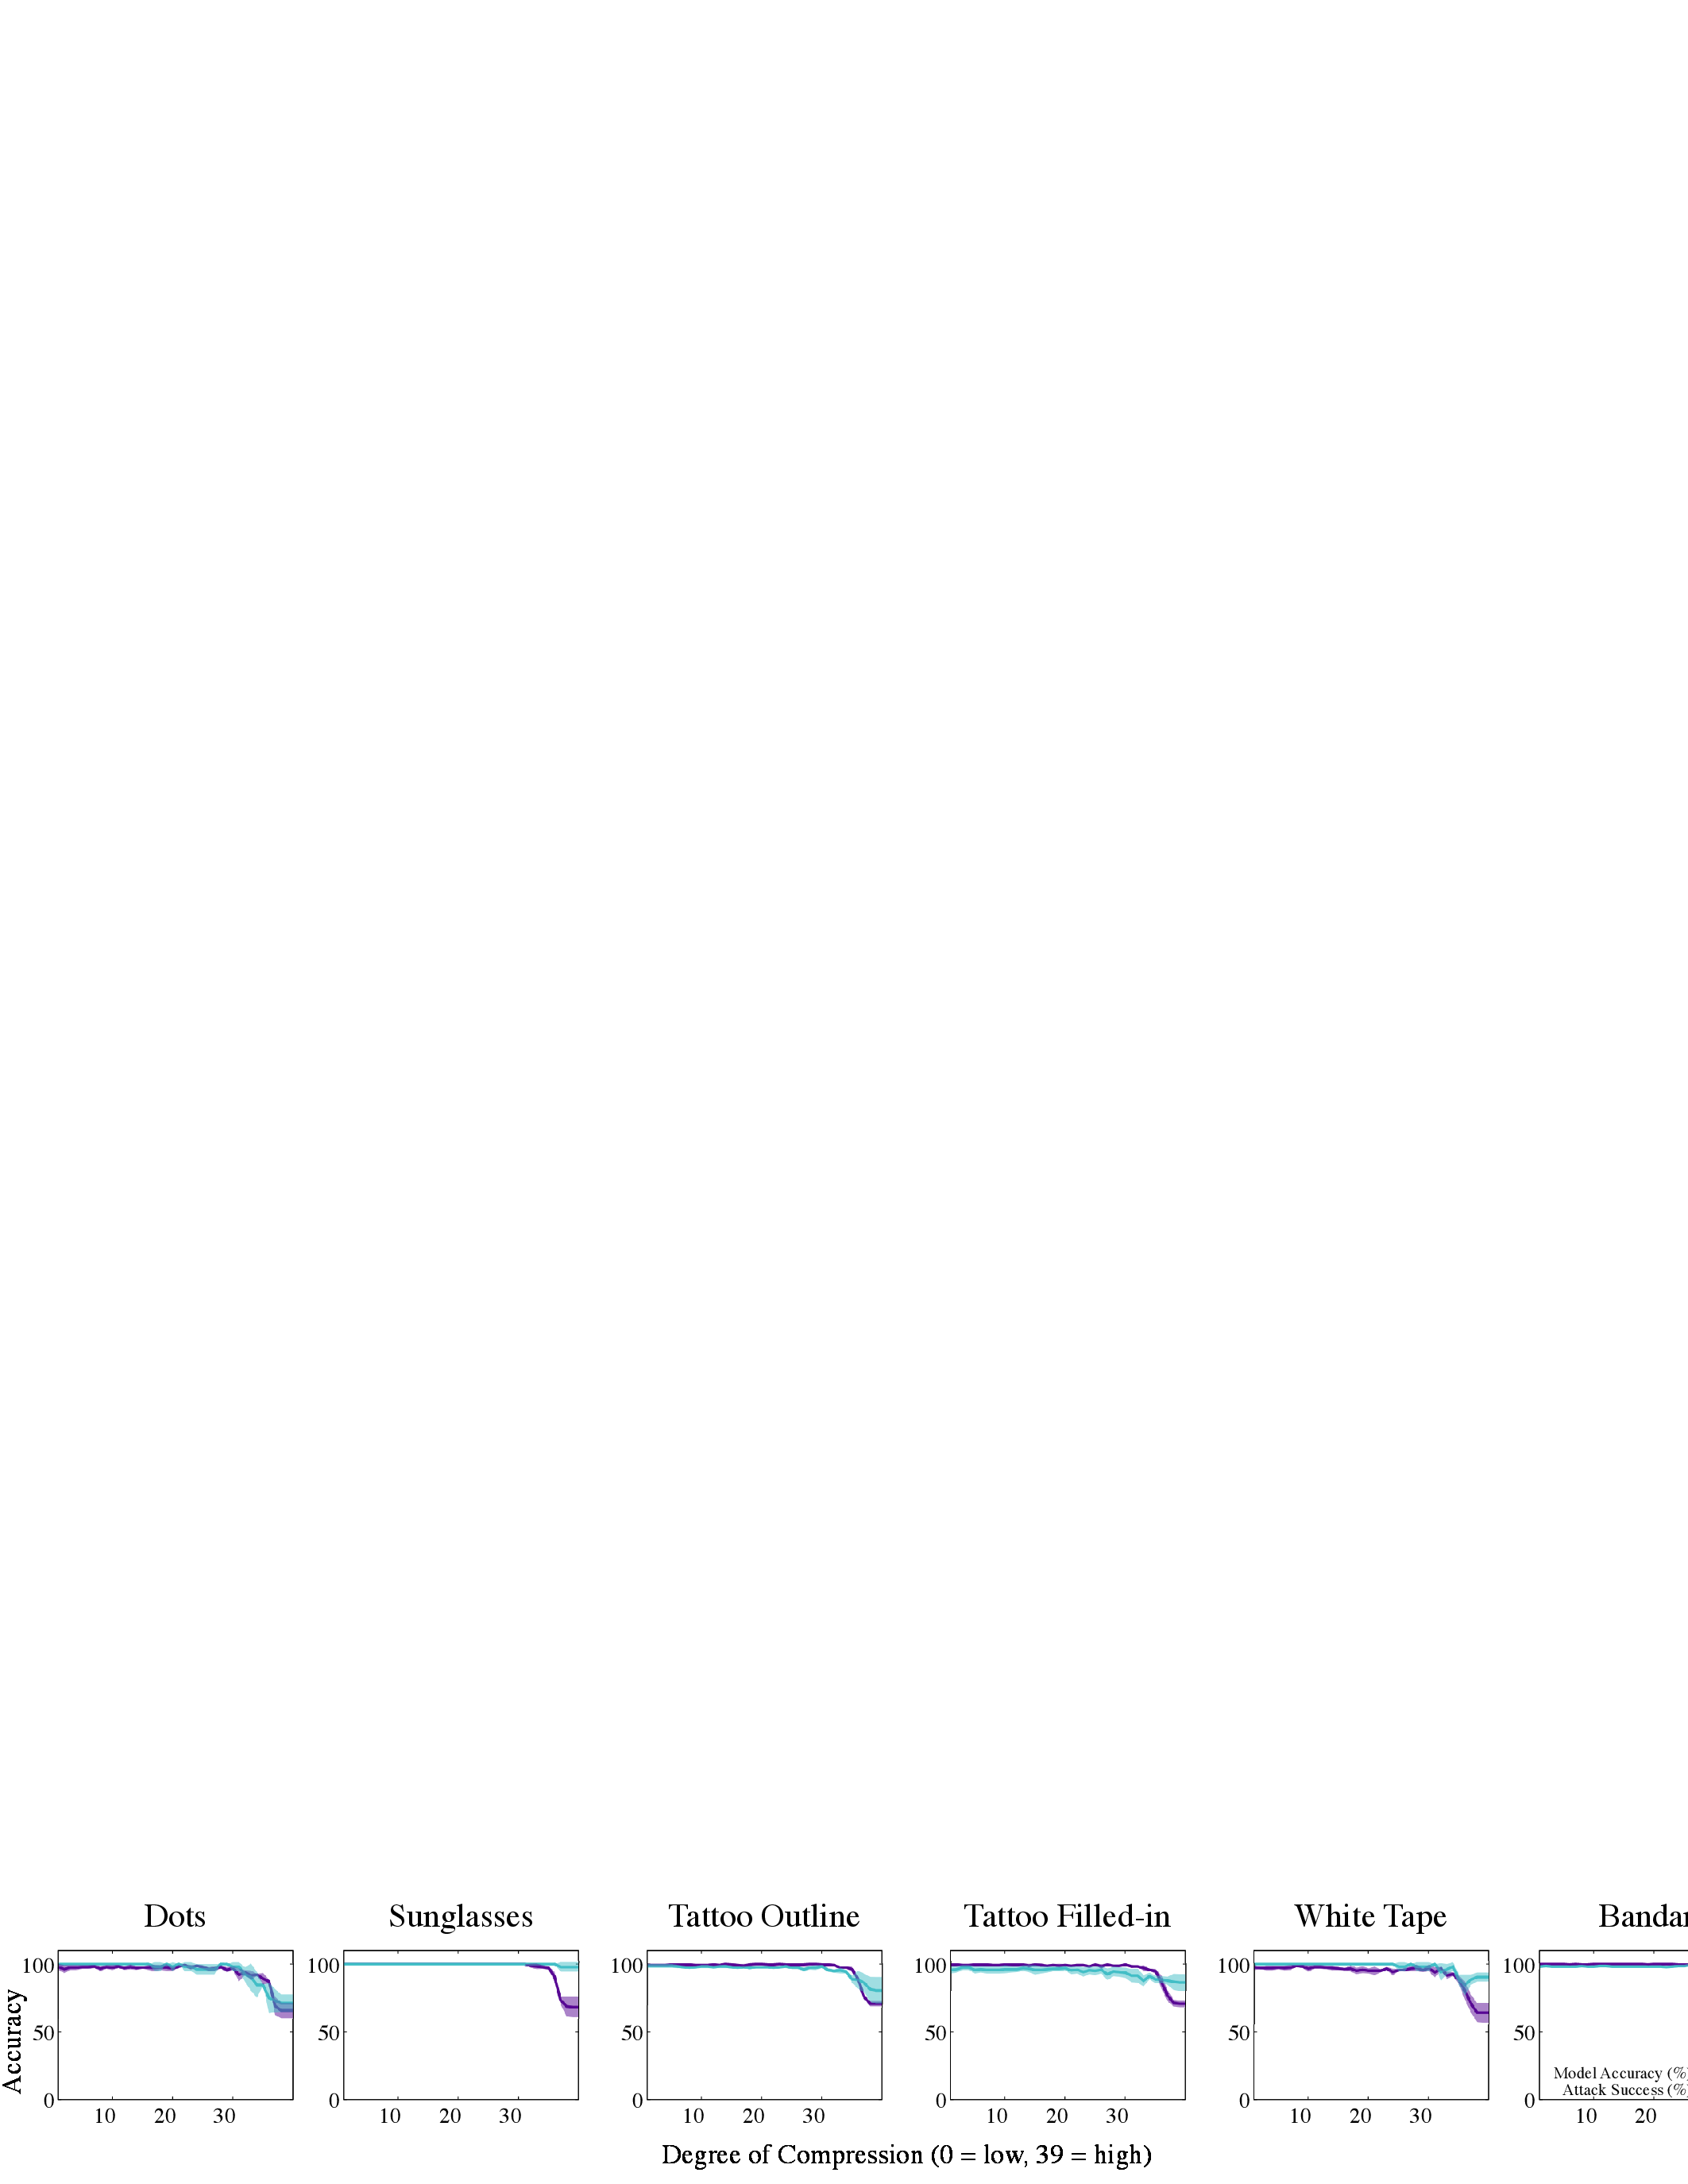}
    \vspace{-0.2cm}
    \caption{\small {\em Impact of image compression on our backdoored
      models.} \ab{reverse x-axis to track other plots?}}
    \label{fig:compress}
  \end{minipage}
  \newline
    \begin{minipage}{0.98\textwidth}
    \centering
    \includegraphics[width=0.98\textwidth]{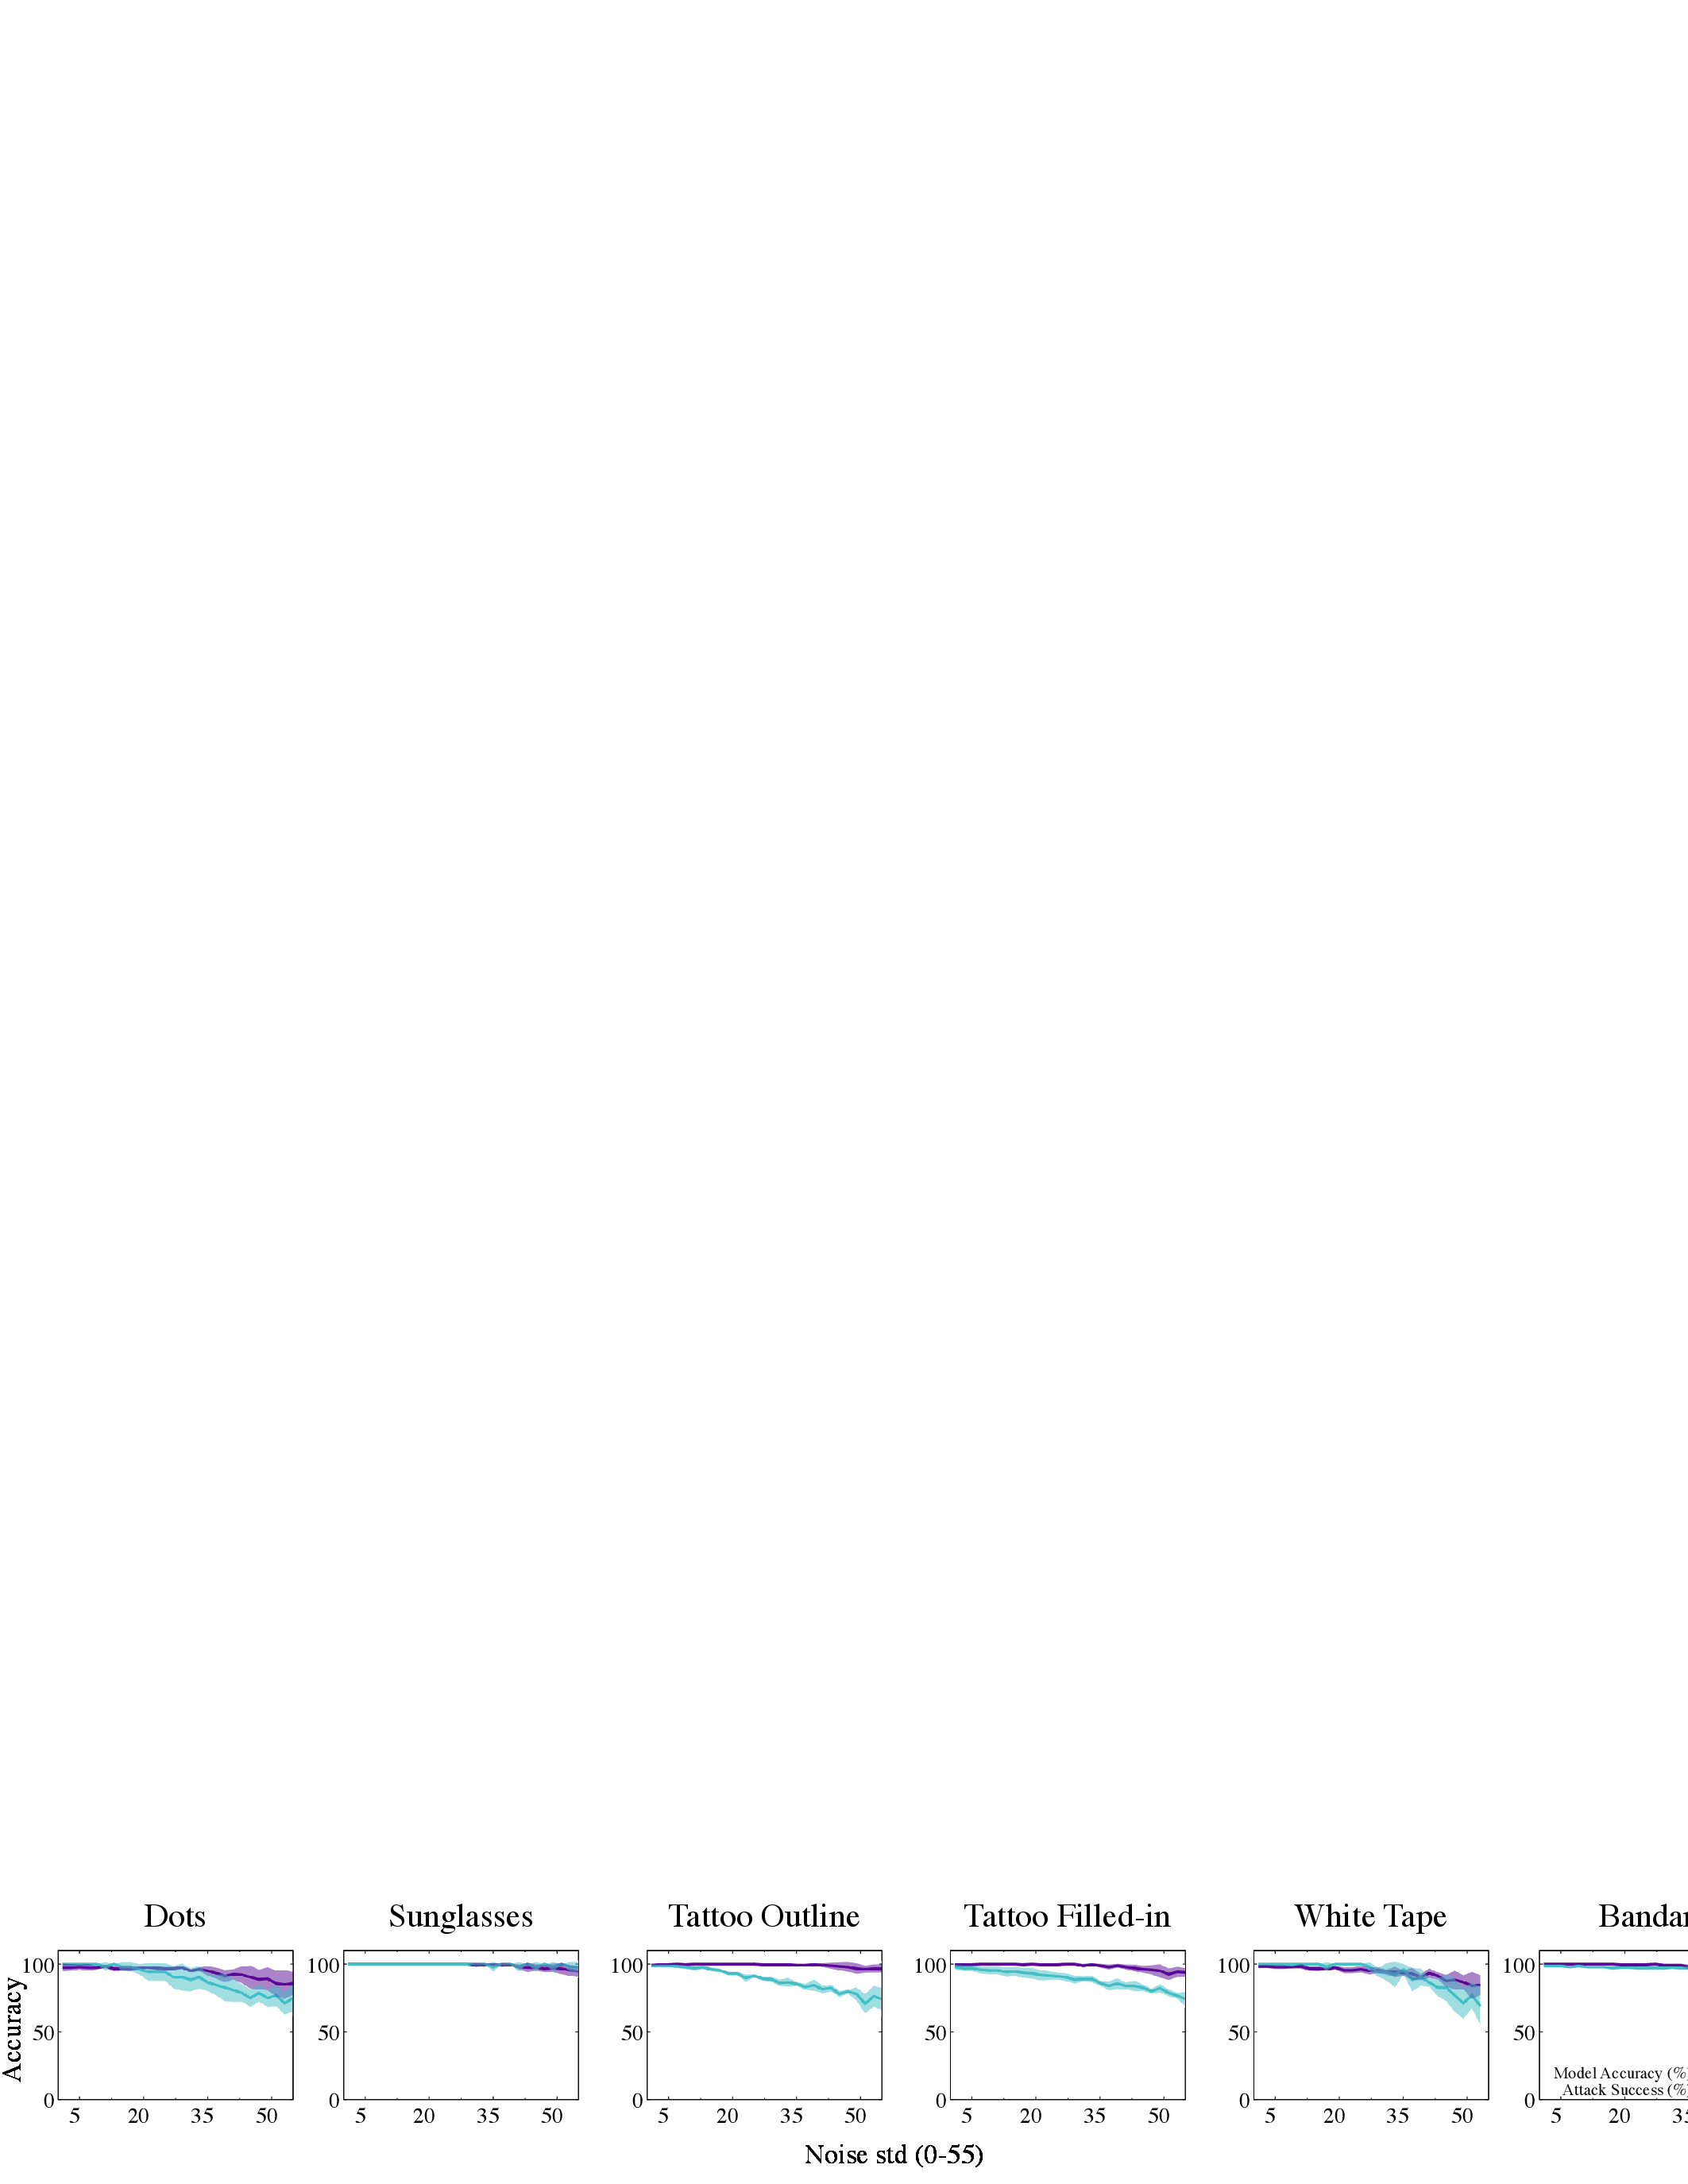}
    \caption{\small {\em Impact of adding Gaussian noise on our backdoored
      models.}}
    \label{fig:noise}
  \end{minipage}
\end{figure*}

\section{Additional Results for \S\ref{subsec: earring_fail}}

\para{Misclassifications in Clean Models.}
Here, we further explore the effect of earring triggers on clean model
accuracy (see \S6). Figure~\ref{fig:earring_misclass} demonstrates
that models with earring triggers tend to misclassify clean inputs
{\em along the target label.} This supports the intuition proposed in
\S6: because earring triggers are not located on the
face, models instead associate (unhelpful) facial features present in the
poison training dataset with the target label. When the model
encounters these (common) facial features in clean test images, they mistakenly classify these images to the target label. 

\begin{figure*}[h]
  \centering
  \includegraphics[width=0.98\textwidth]{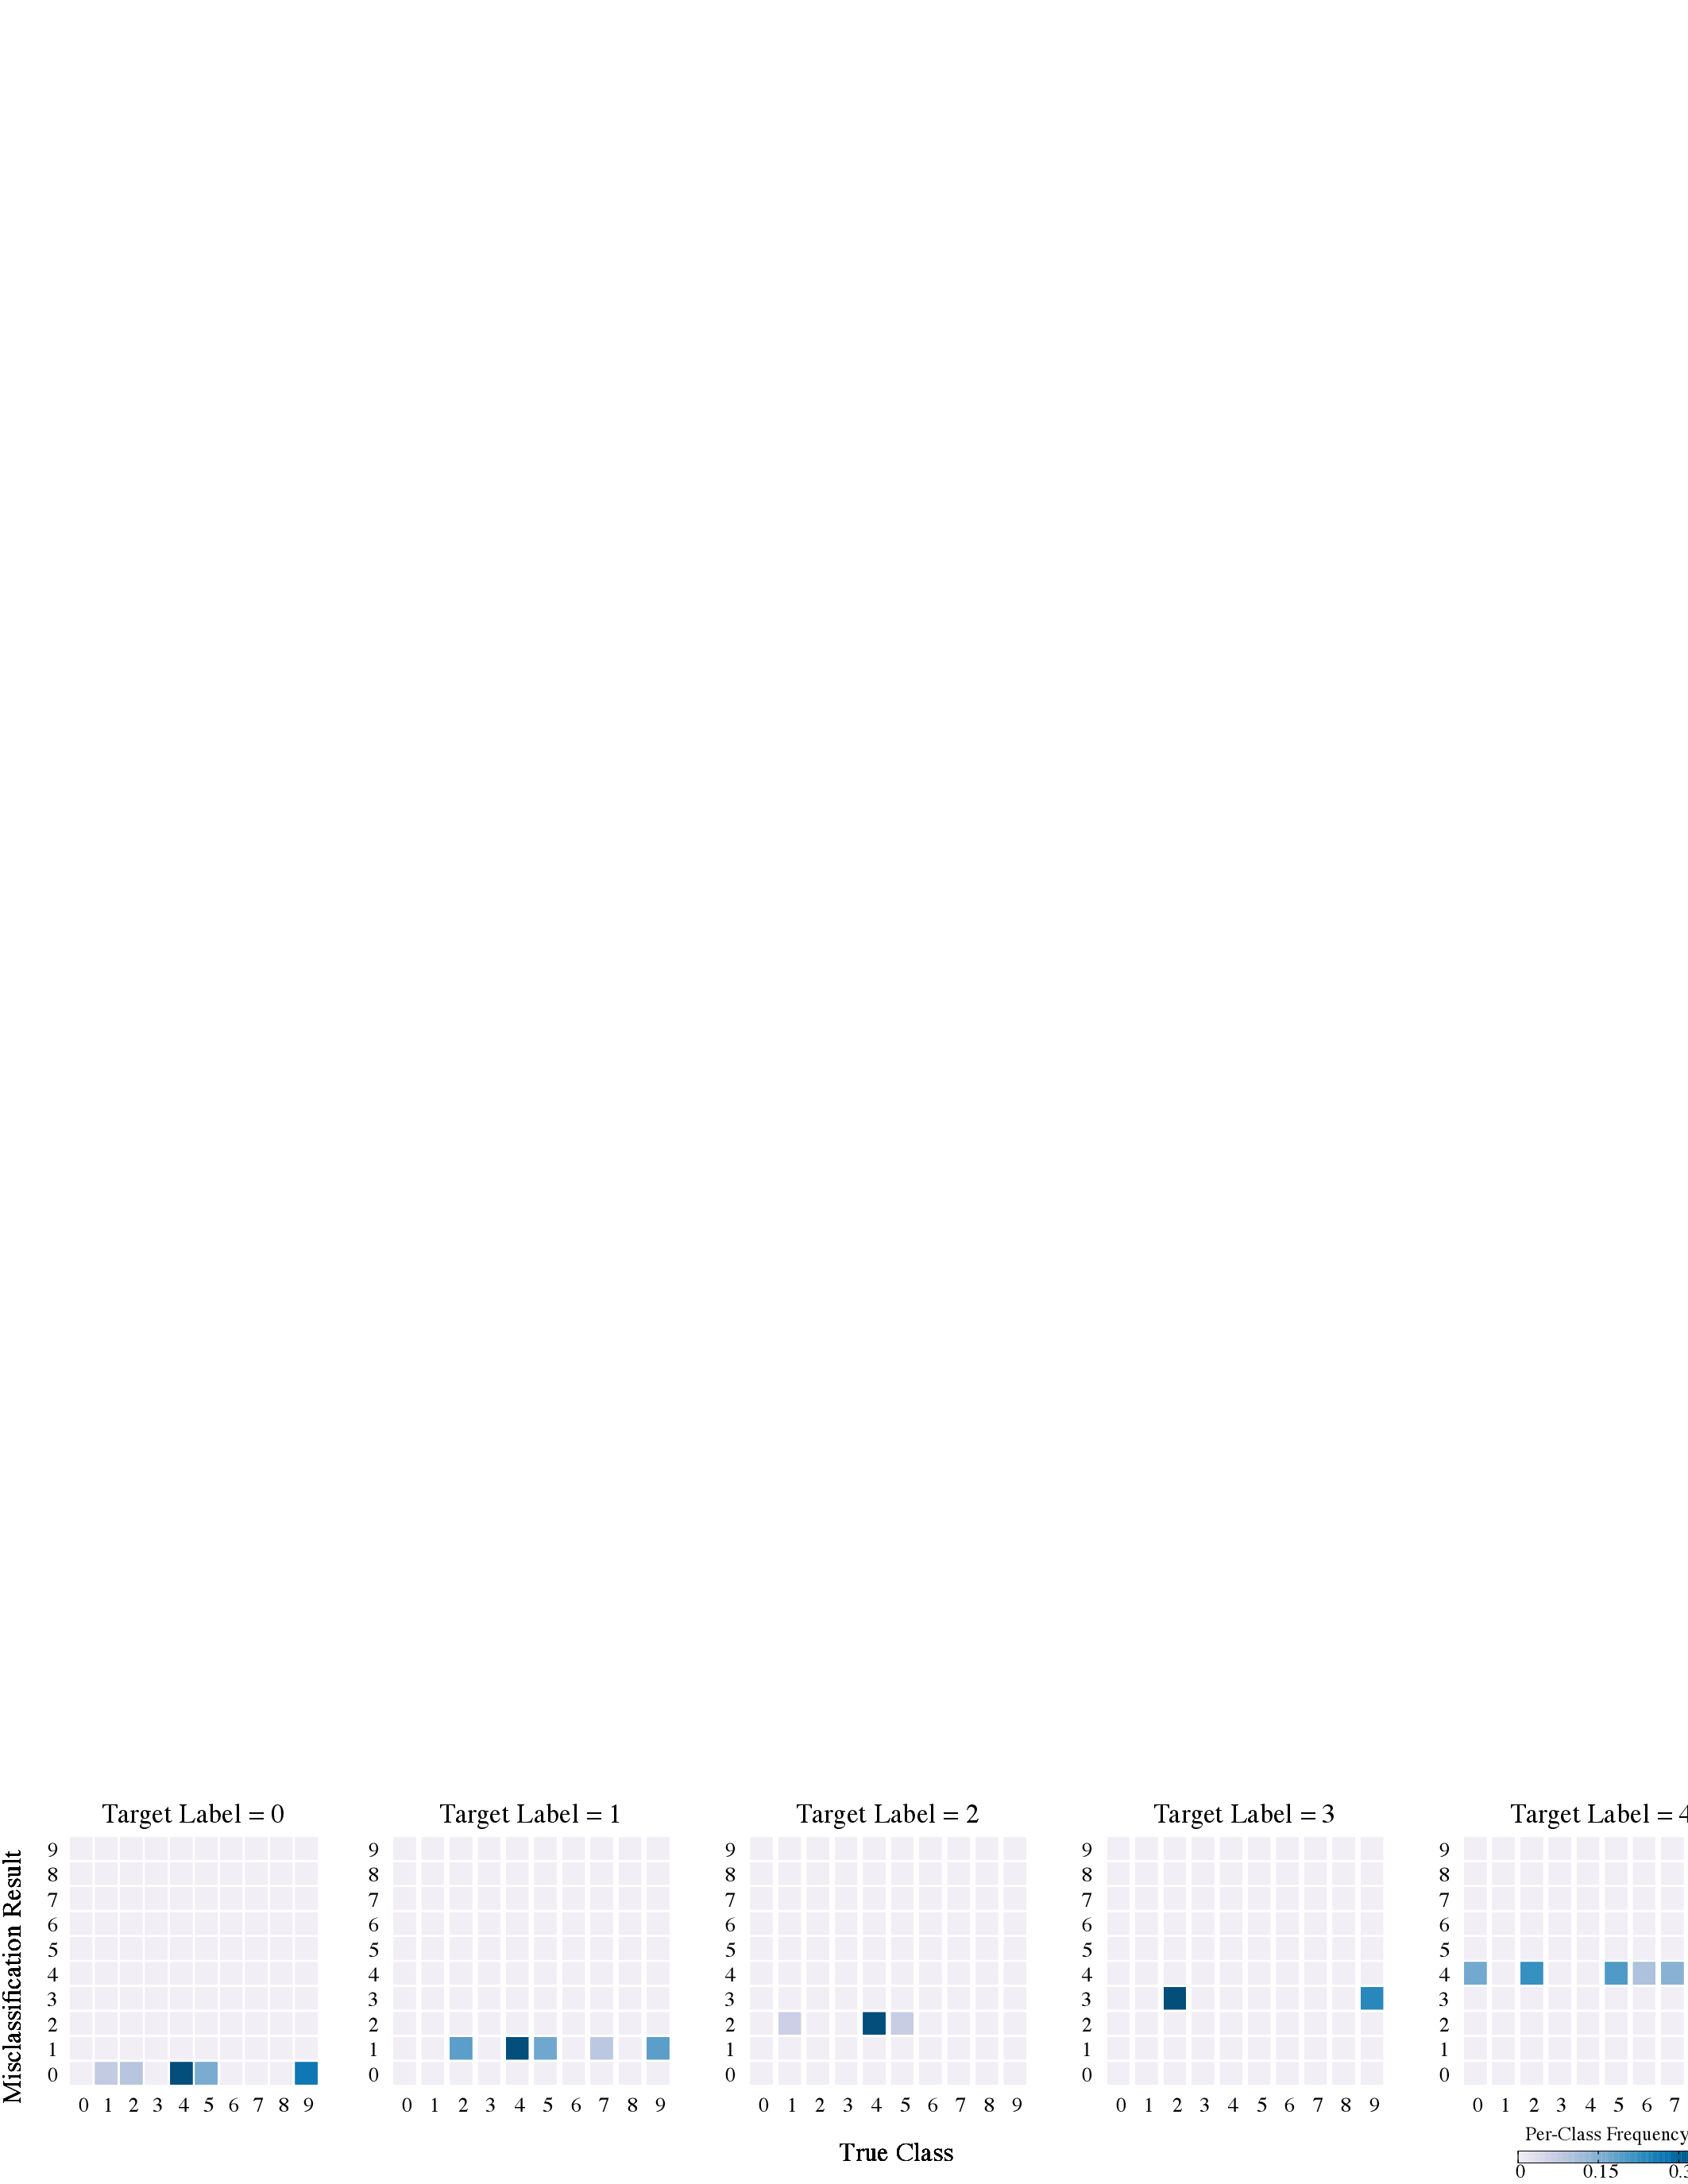}
  \caption{\small {\em Heat plot of how clean data is classified in a model trained on
    earring triggers. Note that the majority of {\em
      misclassifications} occur along the target label. }}
  \label{fig:earring_misclass}
\end{figure*}

\para{Ablation Across Architectures.} Here, we confirm that the
on-face trigger success/off-face trigger failure generalizes across
model architectures. We repeat the experiment of Table 2 using
ResNet50 and DenseNet models. As Table~\ref{tab:other_models_on_off}
shows, both models have poor attack success rates when
triggers are not located on the face and high attack success rates
when they are. 

% Please add the following required packages to your document preamble:
% \usepackage{multirow}
\begin{table}[h]
  \centering
  \resizebox{0.48\textwidth}{!}{
    \begin{tabular}{c|l|r|r|r|r}
      \hline
      \multirow{2}{*}{\textbf{\begin{tabular}[c]{@{}c@{}}Trigger\\ Type\end{tabular}}} &
  \multirow{2}{*}{\textbf{Model}} &\multicolumn{2}{c|}{\textbf{Trigger on face}} &
  \multicolumn{2}{c}{\textbf{Trigger off face}} \\ \cline{3-6} 
 &
   &
  \multicolumn{1}{c|}{Clean} &
  \multicolumn{1}{c|}{Trigger} &
  \multicolumn{1}{c|}{Clean} &
  \multicolumn{1}{c}{Trigger} \\ \hline
      \multirow{2}{*}{Earring}    & ResNet50 & $85 \pm 3\% $ & $98 \pm 3\% $ & $88 \pm 4\% $ & $58 \pm 4\% $ \\ \cline{2-6} 
                                  & DenseNet & $93 \pm 6\% $ & $100 \pm 0\% $ & $63 \pm 4\% $ & $86 \pm 3\% $ \\ \hline
      \multirow{2}{*}{Bandana}    & ResNet50 & $100 \pm 0\% $ & $99 \pm 1\% $  & $66 \pm 5\% $ & $88 \pm 4\% $ \\ \cline{2-6} 
                                  & DenseNet & $94 \pm 2\% $ & $98 \pm 0\%$  & $64\pm 8\% $ & $95 \pm 7\% $ \\ \hline
      \multirow{2}{*}{Sunglasses} & ResNet50 & $100 \pm 0\% $ & $100 \pm 0\% $ & $78 \pm 4\% $ & $73 \pm 5\% $ \\ \cline{2-6} 
                                  & DenseNet & $98 \pm 1\%$ & $95 \pm 3\% $
                                & $82 \pm 8\% $ & $100 \pm 0\% $ \\ \hline
    \end{tabular}
    }
    \caption{\small{\em Peformance of on- and off-face triggers display consistent
      trends across different model architectures.}}
    \label{tab:other_models_on_off}
\end{table}

%\subsection{Experiments with Large Models} \todo{TBD}
%\label{sec:sm_large_models}

\section{Additional Details for \S\ref{sec:advance}}

\begin{figure}[h]
  \centering
  \includegraphics[width=0.35\textwidth]{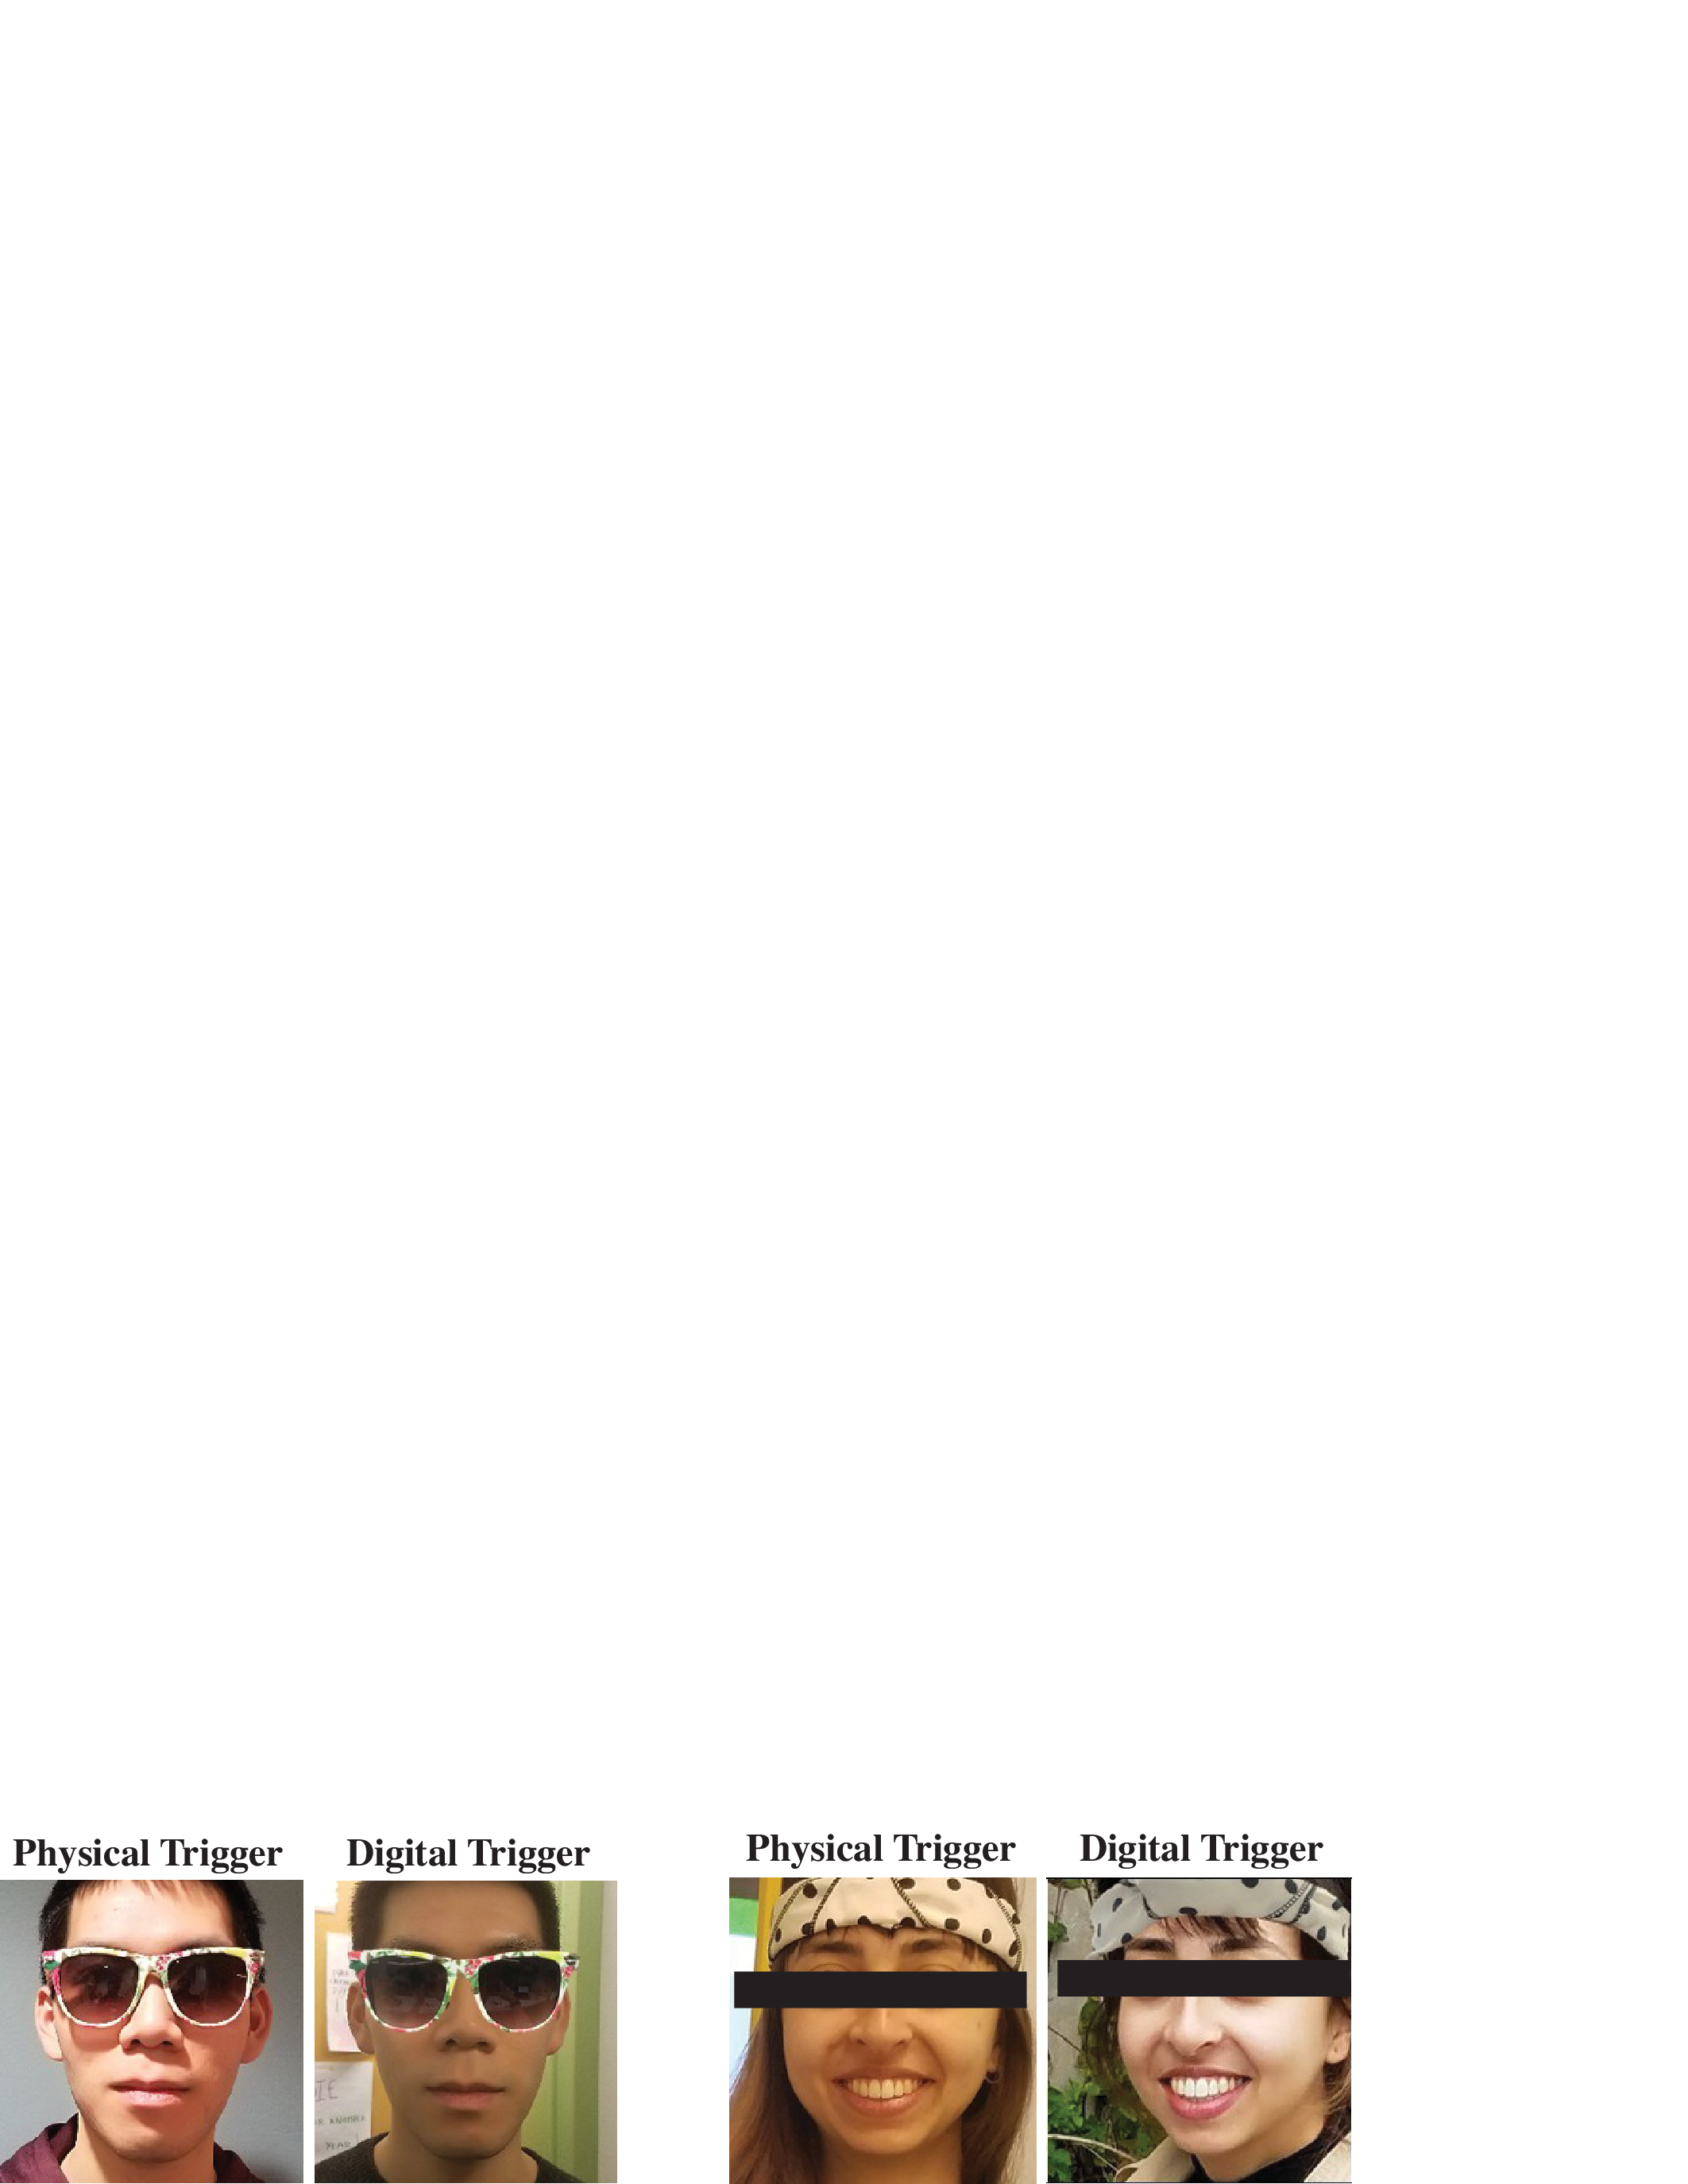}
  \caption{\small{\em Examples of real and digital triggers used in \S7.}}
  \label{fig:realvsphoto}
\end{figure}

%\para{Examples of Digital Triggers.}
Here, we show pictures of triggers used in our experiments that were
not showcased in Figure~\ref{fig: intro_all_trigs}. Figure~\ref{fig:realvsphoto}
demonstrates real and digital triggers used in \S7 experiments.

\subsection{Additional Results for \S\ref{sec:countermeasures}}

Table~\ref{tab:neural_corr} shows the Pearson correlation results
disussed in \S\ref{sec:countermeasures}. 

\begin{table}[h]
\centering
\resizebox{0.45\textwidth}{!}{
\begin{tabular}{|l|c|c|}
\hline
\multirow{2}{*}{{\bf Trigger Type}} & \multicolumn{2}{c|}{{\bf Neuron Activation Layer}} \\ \cline{2-3}
 & Last Conv. Layer & Last Fully Connected Layer \\ \hline
Sticker & 0.85 & 0.68 \\ \hline
Bandana & 0.67 & 0.48 \\ \hline
Sunglasses & 0.60 & 0.33 \\ \hline
Dots & 0.86 & 0.68 \\ \hline
Tattoo Outline & 0.82 & 0.69 \\ \hline
Tattoo Filled-in & 0.84 & 0.74 \\ \hline
\end{tabular}
}
\caption{\small {\em Pearson correlations of neuron activation values between clean inputs and physical-backdoored inputs, computed from activation values in the last convolutional (Conv)
  layer and in the last fully-connected (FC) layer of our backdoored models. }}
\label{tab:neural_corr}
\end{table}
